# Supplementary material for: A symmetry-preserving and transferable representation for learning the Kohn-Sham density matrix
Source: arXiv:2503.08400 source file (2025-03-11)
Supplement: Supplementary file 1 [file SI.pdf]

# Supporting Information for “A symmetry-preserving and transferable representation for learning the Kohn-Sham density matrix”

Liwei Zhang<sup>1</sup>, Patrizia Mazzeo<sup>2</sup>, Michele Nottoli<sup>3</sup>, Edoardo Cignoni<sup>2</sup>, Lorenzo Cupellini<sup>2</sup>, and Benjamin Stamm<sup>3</sup>

<sup>1</sup>Institut für Geometrie und Praktische Mathematik, RWTH Aachen University,  
Templergraben 55, 52062 Aachen, Germany

<sup>2</sup>Dipartimento di Chimica e Chimica Industriale, Università di Pisa, 56124 Pisa, Italy

<sup>3</sup>Universität Stuttgart, Institute of Applied Analysis and Numerical Simulation,  
Pfaffenwaldring 57, 70569 Stuttgart, Germany

## 1 Additional tables

| Molecule       | Specific Model  |             |                      |                      | Unified Model   |             |                      |                      | Unified Model-A |             |                      |                 | Unified-Alcohol-Model |                      |  |
|----------------|-----------------|-------------|----------------------|----------------------|-----------------|-------------|----------------------|----------------------|-----------------|-------------|----------------------|-----------------|-----------------------|----------------------|--|
|                | training frames | test frames | $r_{\text{cut}}=4.0$ | $r_{\text{cut}}=6.5$ | training frames | test frames | $r_{\text{cut}}=4.0$ | $r_{\text{cut}}=6.5$ | training frames | test frames | $r_{\text{cut}}=4.0$ | training frames | test frames           | $r_{\text{cut}}=4.0$ |  |
| Acetaldehyde   | 0:2999          | 3000:9999   | $4.416\cdot 10^{-5}$ | $4.240\cdot 10^{-5}$ | 0:30:8999       | 9000:9999   | $3.278\cdot 10^{-4}$ | $3.861\cdot 10^{-4}$ | 0:30:8999       | 9000:9999   | $3.299\cdot 10^{-4}$ | -               | -                     | -                    |  |
| Acrolein       | 0:2:5999        | 6000:9999   | $2.514\cdot 10^{-4}$ | $1.409\cdot 10^{-4}$ | 0:30:8999       | 9000:9999   | $5.028\cdot 10^{-4}$ | $4.277\cdot 10^{-4}$ | 0:30:8999       | 9000:9999   | $5.081\cdot 10^{-4}$ | -               | -                     | -                    |  |
| Aniline        | 0:2:2999        | 3000:9999   | $4.300\cdot 10^{-4}$ | $1.634\cdot 10^{-4}$ | 0:30:8999       | 9000:9999   | $4.868\cdot 10^{-4}$ | $3.177\cdot 10^{-4}$ | 0:30:8999       | 9000:9999   | $4.876\cdot 10^{-4}$ | -               | -                     | -                    |  |
| o-Toluidine    | 0:2:2999        | 3000:9999   | $5.430\cdot 10^{-4}$ | $2.738\cdot 10^{-4}$ | 0:30:8999       | 9000:9999   | $5.962\cdot 10^{-4}$ | $3.584\cdot 10^{-4}$ | 0:30:8999       | 9000:9999   | $5.940\cdot 10^{-4}$ | -               | -                     | -                    |  |
| m-Toluidine    | 0:2:2999        | 3000:9999   | $5.384\cdot 10^{-4}$ | $2.596\cdot 10^{-4}$ | 0:30:8999       | 9000:9999   | $5.824\cdot 10^{-4}$ | $3.727\cdot 10^{-4}$ | 0:30:8999       | 9000:9999   | $5.822\cdot 10^{-4}$ | -               | -                     | -                    |  |
| Benzene*       | -               | -           | -                    | -                    | -               | 0:99        | $4.058\cdot 10^{-4}$ | $8.638\cdot 10^{-3}$ | -               | 0:99        | $3.646\cdot 10^{-4}$ | -               | -                     | -                    |  |
| Toluene*       | -               | -           | -                    | -                    | -               | 0:99        | $6.369\cdot 10^{-4}$ | $7.674\cdot 10^{-3}$ | -               | 0:99        | $5.980\cdot 10^{-4}$ | -               | -                     | -                    |  |
| Phenol**       | -               | -           | -                    | -                    | -               | 0:99        | $4.809\cdot 10^{-3}$ | $1.795\cdot 10^{-2}$ | 0:10:89         | others      | $6.770\cdot 10^{-4}$ | -               | -                     | -                    |  |
| Benzaldehyde** | -               | -           | -                    | -                    | -               | 0:99        | $4.129\cdot 10^{-3}$ | $1.997\cdot 10^{-2}$ | 0:10:89         | others      | $1.201\cdot 10^{-3}$ | -               | -                     | -                    |  |
| p-Toluidine**  | -               | -           | -                    | -                    | -               | 0:99        | $2.840\cdot 10^{-3}$ | $1.907\cdot 10^{-3}$ | 0:10:89         | others      | $6.293\cdot 10^{-4}$ | -               | -                     | -                    |  |
| Propanol       | 0:2999          | 3000:9999   | $3.049\cdot 10^{-4}$ | $2.421\cdot 10^{-4}$ | 0:30:8999       | 9000:9999   | $4.427\cdot 10^{-4}$ | $4.080\cdot 10^{-4}$ | 0:30:8999       | 9000:9999   | $4.444\cdot 10^{-4}$ | 0:24:8999       | 9000:9999             | $3.932\cdot 10^{-4}$ |  |
| Butanol        | 0:3:8999        | 9000:9999   | $4.510\cdot 10^{-4}$ | $7.643\cdot 10^{-4}$ | 0:30:8999       | 9000:9999   | $4.921\cdot 10^{-4}$ | $1.273\cdot 10^{-3}$ | 0:30:8999       | 9000:9999   | $4.934\cdot 10^{-4}$ | 0:24:8999       | 9000:9999             | $4.477\cdot 10^{-4}$ |  |
| 2-Butanol      | 0:2999          | 3000:9999   | $9.173\cdot 10^{-4}$ | $7.603\cdot 10^{-4}$ | 0:30:8999       | 9000:9999   | $1.494\cdot 10^{-3}$ | $6.581\cdot 10^{-4}$ | 0:30:8999       | 9000:9999   | $1.509\cdot 10^{-3}$ | 0:24:8999       | 9000:9999             | $7.598\cdot 10^{-4}$ |  |
| Hexanol        | 0:2:2999        | 3000:9999   | $1.031\cdot 10^{-3}$ | $7.021\cdot 10^{-4}$ | 0:30:8999       | 9000:9999   | $5.423\cdot 10^{-4}$ | $9.614\cdot 10^{-4}$ | 0:30:8999       | 9000:9999   | $5.314\cdot 10^{-4}$ | 0:24:8999       | 9000:9999             | $4.602\cdot 10^{-4}$ |  |
| Ethanol*       | -               | -           | -                    | -                    | -               | 0:99        | $9.644\cdot 10^{-4}$ | $1.021\cdot 10^{-3}$ | -               | 0:99        | $8.999\cdot 10^{-4}$ | -               | 0:99                  | $5.556\cdot 10^{-4}$ |  |
| 2-Propanol*    | -               | -           | -                    | -                    | -               | 0:99        | $7.701\cdot 10^{-4}$ | $7.573\cdot 10^{-4}$ | -               | 0:99        | $7.480\cdot 10^{-4}$ | -               | 0:99                  | $4.686\cdot 10^{-4}$ |  |
| 2-Hexanol*     | -               | -           | -                    | -                    | -               | 0:99        | $7.384\cdot 10^{-4}$ | $4.853\cdot 10^{-3}$ | -               | 0:99        | $7.353\cdot 10^{-4}$ | -               | 0:99                  | $5.485\cdot 10^{-4}$ |  |
| Heptanol*      | -               | -           | -                    | -                    | -               | 0:99        | $8.896\cdot 10^{-4}$ | $1.538\cdot 10^{-3}$ | -               | 0:99        | $8.980\cdot 10^{-4}$ | -               | 0:99                  | $7.048\cdot 10^{-4}$ |  |

Table S1: test set RMSEs for different molecules obtained by (3,8)-models trained with different datasets. In the table, when “-” appears, it means that the corresponding molecule is not included in the training process, and hence there is no dedicated model for these molecules.

| Molecule     | Tol.      | Default guess  | Specific Model                 |                                |
|--------------|-----------|----------------|--------------------------------|--------------------------------|
|              |           |                | $r_{\text{cut}} = 4.0$         | $r_{\text{cut}} = 6.5$         |
| Acetaldehyde | $10^{-6}$ | $9.4 \pm 0.1$  | $5.2 \pm 0.1$ ( $\sim 44\%$ )  | $5.1 \pm 0.1$ ( $\sim 46\%$ )  |
|              | $10^{-7}$ | $12.4 \pm 0.2$ | $7.8 \pm 0.1$ ( $\sim 37\%$ )  | $7.8 \pm 0.1$ ( $\sim 37\%$ )  |
|              | $10^{-8}$ | $14.9 \pm 0.1$ | $9.8 \pm 0.1$ ( $\sim 34\%$ )  | $9.7 \pm 0.1$ ( $\sim 35\%$ )  |
| Acrolein     | $10^{-6}$ | $10.5 \pm 0.1$ | $7.5 \pm 0.2$ ( $\sim 29\%$ )  | $6.3 \pm 0.2$ ( $\sim 40\%$ )  |
|              | $10^{-7}$ | $13.4 \pm 0.1$ | $9.8 \pm 0.1$ ( $\sim 26\%$ )  | $9.1 \pm 0.1$ ( $\sim 32\%$ )  |
|              | $10^{-8}$ | $16.0 \pm 0.2$ | $11.5 \pm 0.1$ ( $\sim 28\%$ ) | $11.2 \pm 0.1$ ( $\sim 30\%$ ) |
| Aniline      | $10^{-6}$ | $9.9 \pm 0.1$  | $7.2 \pm 0.1$ ( $\sim 28\%$ )  | $6.5 \pm 0.1$ ( $\sim 35\%$ )  |
|              | $10^{-7}$ | $12.5 \pm 0.1$ | $9.7 \pm 0.1$ ( $\sim 23\%$ )  | $8.7 \pm 0.1$ ( $\sim 31\%$ )  |
|              | $10^{-8}$ | $14.7 \pm 0.1$ | $11.9 \pm 0.1$ ( $\sim 19\%$ ) | $11.1 \pm 0.1$ ( $\sim 24\%$ ) |
| o-Toluidine  | $10^{-6}$ | $10.0 \pm 0.0$ | $7.6 \pm 0.1$ ( $\sim 24\%$ )  | $7.2 \pm 0.1$ ( $\sim 28\%$ )  |
|              | $10^{-7}$ | $12.8 \pm 0.1$ | $9.9 \pm 0.1$ ( $\sim 22\%$ )  | $9.7 \pm 0.1$ ( $\sim 24\%$ )  |
|              | $10^{-8}$ | $14.9 \pm 0.0$ | $12.3 \pm 0.1$ ( $\sim 18\%$ ) | $11.7 \pm 0.1$ ( $\sim 22\%$ ) |
| m-Toluidine  | $10^{-6}$ | $10.0 \pm 0.0$ | $7.3 \pm 0.1$ ( $\sim 27\%$ )  | $7.1 \pm 0.1$ ( $\sim 29\%$ )  |
|              | $10^{-7}$ | $12.7 \pm 0.1$ | $9.8 \pm 0.1$ ( $\sim 23\%$ )  | $9.5 \pm 0.1$ ( $\sim 25\%$ )  |
|              | $10^{-8}$ | $14.8 \pm 0.1$ | $11.9 \pm 0.1$ ( $\sim 19\%$ ) | $11.7 \pm 0.1$ ( $\sim 21\%$ ) |
| 1-Propanol   | $10^{-6}$ | $9.0 \pm 0.0$  | $6.0 \pm 0.1$ ( $\sim 33\%$ )  | $6.0 \pm 0.1$ ( $\sim 33\%$ )  |
|              | $10^{-7}$ | $11.0 \pm 0.1$ | $8.0 \pm 0.0$ ( $\sim 27\%$ )  | $8.0 \pm 0.0$ ( $\sim 27\%$ )  |
|              | $10^{-8}$ | $13.2 \pm 0.1$ | $9.8 \pm 0.1$ ( $\sim 25\%$ )  | $9.8 \pm 0.1$ ( $\sim 26\%$ )  |
| 1-Butanol    | $10^{-6}$ | $9.0 \pm 0.0$  | $6.4 \pm 0.1$ ( $\sim 29\%$ )  | $6.4 \pm 0.1$ ( $\sim 29\%$ )  |
|              | $10^{-7}$ | $11.0 \pm 0.0$ | $8.1 \pm 0.1$ ( $\sim 27\%$ )  | $8.2 \pm 0.1$ ( $\sim 26\%$ )  |
|              | $10^{-8}$ | $13.2 \pm 0.1$ | $10.1 \pm 0.1$ ( $\sim 24\%$ ) | $10.2 \pm 0.1$ ( $\sim 23\%$ ) |
| 2-Butanol    | $10^{-6}$ | $9.0 \pm 0.0$  | $7.2 \pm 0.1$ ( $\sim 20\%$ )  | $7.5 \pm 0.1$ ( $\sim 16\%$ )  |
|              | $10^{-7}$ | $11.1 \pm 0.1$ | $9.0 \pm 0.1$ ( $\sim 19\%$ )  | $9.3 \pm 0.1$ ( $\sim 16\%$ )  |
|              | $10^{-8}$ | $13.2 \pm 0.1$ | $10.9 \pm 0.1$ ( $\sim 18\%$ ) | $11.0 \pm 0.1$ ( $\sim 17\%$ ) |
| 1-Hexanol    | $10^{-6}$ | $9.0 \pm 0.0$  | $6.4 \pm 0.1$ ( $\sim 29\%$ )  | $6.6 \pm 0.1$ ( $\sim 27\%$ )  |
|              | $10^{-7}$ | $10.9 \pm 0.1$ | $8.2 \pm 0.1$ ( $\sim 24\%$ )  | $8.3 \pm 0.1$ ( $\sim 23\%$ )  |
|              | $10^{-8}$ | $13.0 \pm 0.0$ | $10.3 \pm 0.1$ ( $\sim 21\%$ ) | $10.4 \pm 0.1$ ( $\sim 20\%$ ) |

Table S2: Average of the number of iterations obtained using the predicted density matrix as guess for the calculation on the same geometry. The results refer to the (3,8)-models trained targeting the density matrix. The first column specifies the molecule, the second column indicates the convergence tolerance for the SCF procedure, the third column reports the average of the number of iterations obtained using the default guess available in the Gaussian program and in the last two columns we report the average number of iterations obtained with our predicted density matrix as guess, using the specific model for each molecule and with 4.0 and 6.5 radius of cutoff, respectively. The values reported in parentheses indicate the percentage of reduction with respect to the iterations required by the default guess to converge.

| Molecule     | Tol.      | Default guess  | Specific Model                 |                                |
|--------------|-----------|----------------|--------------------------------|--------------------------------|
|              |           |                | $r_{\text{cut}} = 4.0$         | $r_{\text{cut}} = 6.5$         |
| Acetaldehyde | $10^{-6}$ | $9.4 \pm 0.1$  | $4.8 \pm 0.1$ ( $\sim 49\%$ )  | $4.7 \pm 0.1$ ( $\sim 50\%$ )  |
|              | $10^{-7}$ | $12.4 \pm 0.2$ | $7.3 \pm 0.2$ ( $\sim 41\%$ )  | $7.3 \pm 0.2$ ( $\sim 41\%$ )  |
|              | $10^{-8}$ | $14.9 \pm 0.1$ | $9.3 \pm 0.1$ ( $\sim 38\%$ )  | $9.2 \pm 0.1$ ( $\sim 38\%$ )  |
| Acrolein     | $10^{-6}$ | $10.5 \pm 0.1$ | $7.2 \pm 0.2$ ( $\sim 32\%$ )  | $5.9 \pm 0.2$ ( $\sim 44\%$ )  |
|              | $10^{-7}$ | $13.4 \pm 0.1$ | $9.6 \pm 0.1$ ( $\sim 29\%$ )  | $8.6 \pm 0.1$ ( $\sim 36\%$ )  |
|              | $10^{-8}$ | $16.0 \pm 0.2$ | $11.2 \pm 0.1$ ( $\sim 30\%$ ) | $10.8 \pm 0.1$ ( $\sim 32\%$ ) |
| Aniline      | $10^{-6}$ | $9.9 \pm 0.1$  | $7.0 \pm 0.1$ ( $\sim 29\%$ )  | $6.3 \pm 0.1$ ( $\sim 36\%$ )  |
|              | $10^{-7}$ | $12.5 \pm 0.1$ | $9.4 \pm 0.2$ ( $\sim 25\%$ )  | $8.8 \pm 0.2$ ( $\sim 30\%$ )  |
|              | $10^{-8}$ | $14.7 \pm 0.1$ | $11.7 \pm 0.2$ ( $\sim 20\%$ ) | $11.0 \pm 0.2$ ( $\sim 25\%$ ) |
| o-Toluidine  | $10^{-6}$ | $10.0 \pm 0.0$ | $7.0 \pm 0.1$ ( $\sim 30\%$ )  | $6.9 \pm 0.1$ ( $\sim 31\%$ )  |
|              | $10^{-7}$ | $12.8 \pm 0.1$ | $9.6 \pm 0.1$ ( $\sim 25\%$ )  | $9.4 \pm 0.1$ ( $\sim 27\%$ )  |
|              | $10^{-8}$ | $14.9 \pm 0.0$ | $11.7 \pm 0.1$ ( $\sim 21\%$ ) | $11.4 \pm 0.1$ ( $\sim 24\%$ ) |
| m-Toluidine  | $10^{-6}$ | $10.0 \pm 0.0$ | $7.1 \pm 0.2$ ( $\sim 29\%$ )  | $6.9 \pm 0.2$ ( $\sim 31\%$ )  |
|              | $10^{-7}$ | $12.7 \pm 0.1$ | $9.7 \pm 0.2$ ( $\sim 23\%$ )  | $9.4 \pm 0.2$ ( $\sim 25\%$ )  |
|              | $10^{-8}$ | $14.8 \pm 0.1$ | $11.9 \pm 0.2$ ( $\sim 20\%$ ) | $11.6 \pm 0.2$ ( $\sim 22\%$ ) |
| 1-Propanol   | $10^{-6}$ | $9.0 \pm 0.0$  | $6.0 \pm 0.0$ ( $\sim 33\%$ )  | $5.9 \pm 0.0$ ( $\sim 34\%$ )  |
|              | $10^{-7}$ | $11.0 \pm 0.1$ | $8.0 \pm 0.1$ ( $\sim 27\%$ )  | $7.8 \pm 0.1$ ( $\sim 29\%$ )  |
|              | $10^{-8}$ | $13.2 \pm 0.1$ | $9.9 \pm 0.1$ ( $\sim 25\%$ )  | $9.7 \pm 0.1$ ( $\sim 27\%$ )  |
| 1-Butanol    | $10^{-6}$ | $9.0 \pm 0.0$  | $6.2 \pm 0.1$ ( $\sim 31\%$ )  | $6.2 \pm 0.1$ ( $\sim 32\%$ )  |
|              | $10^{-7}$ | $11.0 \pm 0.0$ | $8.1 \pm 0.1$ ( $\sim 27\%$ )  | $8.1 \pm 0.1$ ( $\sim 27\%$ )  |
|              | $10^{-8}$ | $13.2 \pm 0.1$ | $10.1 \pm 0.1$ ( $\sim 24\%$ ) | $10.0 \pm 0.1$ ( $\sim 24\%$ ) |
| 2-Butanol    | $10^{-6}$ | $9.0 \pm 0.0$  | $7.3 \pm 0.1$ ( $\sim 18\%$ )  | $7.1 \pm 0.1$ ( $\sim 21\%$ )  |
|              | $10^{-7}$ | $11.1 \pm 0.1$ | $9.3 \pm 0.1$ ( $\sim 17\%$ )  | $9.1 \pm 0.1$ ( $\sim 18\%$ )  |
|              | $10^{-8}$ | $13.2 \pm 0.1$ | $11.1 \pm 0.1$ ( $\sim 16\%$ ) | $11.0 \pm 0.1$ ( $\sim 17\%$ ) |
| 1-Hexanol    | $10^{-6}$ | $9.0 \pm 0.0$  | $6.6 \pm 0.1$ ( $\sim 27\%$ )  | $6.7 \pm 0.1$ ( $\sim 25\%$ )  |
|              | $10^{-7}$ | $10.9 \pm 0.1$ | $8.3 \pm 0.1$ ( $\sim 24\%$ )  | $8.6 \pm 0.1$ ( $\sim 21\%$ )  |
|              | $10^{-8}$ | $13.0 \pm 0.0$ | $10.2 \pm 0.1$ ( $\sim 22\%$ ) | $10.4 \pm 0.1$ ( $\sim 20\%$ ) |

Table S3: Average of the number of iterations obtained using the predicted density matrix as guess for the calculation on the same geometry. The results refer to the (3,8)-models trained targeting the Kohn-Sham matrix. The first column specifies the molecule, the second column indicates the convergence tolerance for the SCF procedure, the third column reports the average of the number of iterations obtained using the default guess available in the Gaussian program and in the last two columns we report the average number of iterations obtained with our predicted density matrix as guess, using the specific model for each molecule and with 4.0 and 6.5 radius of cutoff, respectively. The values reported in parentheses indicate the percentage of reduction with respect to the iterations required by the default guess to converge.

| Molecule       | Tol.      | Default guess  | Specific Model                 | Unified Model                  | Unified Model-A                |
|----------------|-----------|----------------|--------------------------------|--------------------------------|--------------------------------|
| Acetaldehyde   | $10^{-6}$ | $9.4 \pm 0.1$  | $5.2 \pm 0.1$ ( $\sim 44\%$ )  | $7.5 \pm 0.1$ ( $\sim 20\%$ )  | $7.5 \pm 0.1$ ( $\sim 20\%$ )  |
|                | $10^{-7}$ | $12.4 \pm 0.2$ | $7.8 \pm 0.1$ ( $\sim 37\%$ )  | $9.7 \pm 0.1$ ( $\sim 22\%$ )  | $9.7 \pm 0.1$ ( $\sim 22\%$ )  |
|                | $10^{-8}$ | $14.9 \pm 0.1$ | $9.8 \pm 0.1$ ( $\sim 34\%$ )  | $11.1 \pm 0.1$ ( $\sim 26\%$ ) | $11.1 \pm 0.1$ ( $\sim 25\%$ ) |
| Acrolein       | $10^{-6}$ | $10.5 \pm 0.1$ | $7.5 \pm 0.2$ ( $\sim 29\%$ )  | $8.3 \pm 0.2$ ( $\sim 21\%$ )  | $8.3 \pm 0.2$ ( $\sim 21\%$ )  |
|                | $10^{-7}$ | $13.4 \pm 0.1$ | $9.8 \pm 0.1$ ( $\sim 26\%$ )  | $10.5 \pm 0.1$ ( $\sim 22\%$ ) | $10.5 \pm 0.1$ ( $\sim 21\%$ ) |
|                | $10^{-8}$ | $16.0 \pm 0.2$ | $11.5 \pm 0.1$ ( $\sim 28\%$ ) | $12.0 \pm 0.1$ ( $\sim 25\%$ ) | $12.1 \pm 0.1$ ( $\sim 24\%$ ) |
| Aniline        | $10^{-6}$ | $9.9 \pm 0.1$  | $7.2 \pm 0.1$ ( $\sim 28\%$ )  | $7.5 \pm 0.1$ ( $\sim 24\%$ )  | $7.5 \pm 0.1$ ( $\sim 24\%$ )  |
|                | $10^{-7}$ | $12.5 \pm 0.1$ | $9.7 \pm 0.1$ ( $\sim 23\%$ )  | $9.9 \pm 0.1$ ( $\sim 21\%$ )  | $9.9 \pm 0.1$ ( $\sim 21\%$ )  |
|                | $10^{-8}$ | $14.7 \pm 0.1$ | $11.9 \pm 0.1$ ( $\sim 19\%$ ) | $12.1 \pm 0.1$ ( $\sim 18\%$ ) | $12.1 \pm 0.1$ ( $\sim 18\%$ ) |
| o-Toluidine    | $10^{-6}$ | $10.0 \pm 0.0$ | $7.6 \pm 0.1$ ( $\sim 24\%$ )  | $7.8 \pm 0.1$ ( $\sim 22\%$ )  | $7.8 \pm 0.1$ ( $\sim 22\%$ )  |
|                | $10^{-7}$ | $12.8 \pm 0.1$ | $9.9 \pm 0.1$ ( $\sim 22\%$ )  | $10.1 \pm 0.1$ ( $\sim 21\%$ ) | $10.1 \pm 0.1$ ( $\sim 21\%$ ) |
|                | $10^{-8}$ | $14.9 \pm 0.0$ | $12.3 \pm 0.1$ ( $\sim 18\%$ ) | $12.5 \pm 0.1$ ( $\sim 16\%$ ) | $12.5 \pm 0.1$ ( $\sim 16\%$ ) |
| m-Toluidine    | $10^{-6}$ | $10.0 \pm 0.0$ | $7.3 \pm 0.1$ ( $\sim 27\%$ )  | $7.6 \pm 0.1$ ( $\sim 24\%$ )  | $7.6 \pm 0.1$ ( $\sim 24\%$ )  |
|                | $10^{-7}$ | $12.7 \pm 0.1$ | $9.8 \pm 0.1$ ( $\sim 23\%$ )  | $9.9 \pm 0.1$ ( $\sim 22\%$ )  | $9.9 \pm 0.1$ ( $\sim 22\%$ )  |
|                | $10^{-8}$ | $14.8 \pm 0.1$ | $11.9 \pm 0.1$ ( $\sim 19\%$ ) | $12.1 \pm 0.1$ ( $\sim 18\%$ ) | $12.1 \pm 0.1$ ( $\sim 18\%$ ) |
| Benzene*       | $10^{-6}$ | $9.0 \pm 0.0$  | -                              | $7.4 \pm 0.1$ ( $\sim 18\%$ )  | $7.4 \pm 0.1$ ( $\sim 18\%$ )  |
|                | $10^{-7}$ | $11.3 \pm 0.1$ | -                              | $9.7 \pm 0.1$ ( $\sim 14\%$ )  | $9.7 \pm 0.1$ ( $\sim 14\%$ )  |
|                | $10^{-8}$ | $13.5 \pm 0.1$ | -                              | $11.7 \pm 0.1$ ( $\sim 13\%$ ) | $11.7 \pm 0.1$ ( $\sim 13\%$ ) |
| Toluene*       | $10^{-6}$ | $9.0 \pm 0.0$  | -                              | $8.0 \pm 0.0$ ( $\sim 11\%$ )  | $7.9 \pm 0.1$ ( $\sim 12\%$ )  |
|                | $10^{-7}$ | $11.6 \pm 0.1$ | -                              | $10.1 \pm 0.1$ ( $\sim 13\%$ ) | $10.0 \pm 0.0$ ( $\sim 14\%$ ) |
|                | $10^{-8}$ | $13.9 \pm 0.1$ | -                              | $12.4 \pm 0.1$ ( $\sim 11\%$ ) | $12.3 \pm 0.1$ ( $\sim 12\%$ ) |
| Phenol**       | $10^{-6}$ | $9.9 \pm 0.1$  | -                              | $10.0 \pm 0.1$ ( $\sim -1\%$ ) | $8.1 \pm 0.1$ ( $\sim 18\%$ )  |
|                | $10^{-7}$ | $12.2 \pm 0.1$ | -                              | $12.2 \pm 0.1$ ( $\sim 1\%$ )  | $10.5 \pm 0.1$ ( $\sim 14\%$ ) |
|                | $10^{-8}$ | $14.6 \pm 0.1$ | -                              | $14.4 \pm 0.1$ ( $\sim 2\%$ )  | $12.3 \pm 0.1$ ( $\sim 15\%$ ) |
| Benzaldehyde** | $10^{-6}$ | $10.7 \pm 0.1$ | -                              | $10.5 \pm 0.1$ ( $\sim 2\%$ )  | $9.0 \pm 0.0$ ( $\sim 16\%$ )  |
|                | $10^{-7}$ | $13.2 \pm 0.1$ | -                              | $12.9 \pm 0.0$ ( $\sim 2\%$ )  | $11.5 \pm 0.1$ ( $\sim 14\%$ ) |
|                | $10^{-8}$ | $15.7 \pm 0.1$ | -                              | $15.1 \pm 0.1$ ( $\sim 4\%$ )  | $14.2 \pm 0.1$ ( $\sim 10\%$ ) |
| p-Toluidine**  | $10^{-6}$ | $10.0 \pm 0.0$ | -                              | $8.3 \pm 0.1$ ( $\sim 16\%$ )  | $7.8 \pm 0.1$ ( $\sim 21\%$ )  |
|                | $10^{-7}$ | $12.6 \pm 0.1$ | -                              | $11.1 \pm 0.1$ ( $\sim 12\%$ ) | $10.2 \pm 0.1$ ( $\sim 20\%$ ) |
|                | $10^{-8}$ | $14.9 \pm 0.1$ | -                              | $13.3 \pm 0.1$ ( $\sim 11\%$ ) | $12.6 \pm 0.1$ ( $\sim 15\%$ ) |

Continued on the next page

Table S4: Average of the number of iterations obtained using the predicted density matrix as guess for the calculation on the same geometry. The results refer to the (3,8)-models trained targeting the density matrix ( $r_{\text{cut}} = 4.0$ ). The first column specifies the molecule, the second column indicates the convergence tolerance for the SCF procedure, the third column reports the average of the number of iterations obtained using the default guess available in the Gaussian program and in the last three columns we report the average number of iterations obtained with our predicted density matrix as guess, using the specific models, the unified model and the Unified Model-A, respectively. The values reported in parentheses indicate the percentage of reduction with respect to the iterations required by the default guess to converge. The test molecules with a superscript \* are not included in the training process at all, and those with \*\* are involved in the training of Unified Model-A, with only 10 frames each included.

|             |           |                |                                |                                |                                |
|-------------|-----------|----------------|--------------------------------|--------------------------------|--------------------------------|
| 1-Propanol  | $10^{-6}$ | $9.0 \pm 0.0$  | $6.0 \pm 0.1$ ( $\sim 33\%$ )  | $6.5 \pm 0.1$ ( $\sim 27\%$ )  | $6.5 \pm 0.1$ ( $\sim 28\%$ )  |
|             | $10^{-7}$ | $11.0 \pm 0.1$ | $8.0 \pm 0.0$ ( $\sim 27\%$ )  | $8.1 \pm 0.1$ ( $\sim 26\%$ )  | $8.1 \pm 0.1$ ( $\sim 26\%$ )  |
|             | $10^{-8}$ | $13.2 \pm 0.1$ | $9.8 \pm 0.1$ ( $\sim 25\%$ )  | $10.1 \pm 0.1$ ( $\sim 23\%$ ) | $10.1 \pm 0.1$ ( $\sim 23\%$ ) |
| 1-Butanol   | $10^{-6}$ | $9.0 \pm 0.0$  | $6.4 \pm 0.1$ ( $\sim 29\%$ )  | $6.6 \pm 0.1$ ( $\sim 27\%$ )  | $6.5 \pm 0.1$ ( $\sim 27\%$ )  |
|             | $10^{-7}$ | $11.0 \pm 0.0$ | $8.1 \pm 0.1$ ( $\sim 27\%$ )  | $8.2 \pm 0.1$ ( $\sim 26\%$ )  | $8.2 \pm 0.1$ ( $\sim 26\%$ )  |
|             | $10^{-8}$ | $13.2 \pm 0.1$ | $10.1 \pm 0.1$ ( $\sim 24\%$ ) | $10.2 \pm 0.1$ ( $\sim 23\%$ ) | $10.2 \pm 0.1$ ( $\sim 22\%$ ) |
| 2-Butanol   | $10^{-6}$ | $9.0 \pm 0.0$  | $7.2 \pm 0.1$ ( $\sim 20\%$ )  | $7.0 \pm 0.1$ ( $\sim 22\%$ )  | $7.1 \pm 0.1$ ( $\sim 22\%$ )  |
|             | $10^{-7}$ | $11.1 \pm 0.1$ | $9.0 \pm 0.1$ ( $\sim 19\%$ )  | $8.8 \pm 0.1$ ( $\sim 21\%$ )  | $8.8 \pm 0.1$ ( $\sim 21\%$ )  |
|             | $10^{-8}$ | $13.2 \pm 0.1$ | $10.9 \pm 0.1$ ( $\sim 18\%$ ) | $10.8 \pm 0.1$ ( $\sim 19\%$ ) | $10.8 \pm 0.1$ ( $\sim 19\%$ ) |
| 1-Hexanol   | $10^{-6}$ | $9.0 \pm 0.0$  | $6.4 \pm 0.1$ ( $\sim 29\%$ )  | $6.5 \pm 0.1$ ( $\sim 28\%$ )  | $6.5 \pm 0.1$ ( $\sim 28\%$ )  |
|             | $10^{-7}$ | $10.9 \pm 0.1$ | $8.2 \pm 0.1$ ( $\sim 24\%$ )  | $8.1 \pm 0.1$ ( $\sim 25\%$ )  | $8.2 \pm 0.1$ ( $\sim 25\%$ )  |
|             | $10^{-8}$ | $13.0 \pm 0.0$ | $10.3 \pm 0.1$ ( $\sim 21\%$ ) | $10.2 \pm 0.1$ ( $\sim 21\%$ ) | $10.2 \pm 0.1$ ( $\sim 21\%$ ) |
| Ethanol*    | $10^{-6}$ | $9.1 \pm 0.0$  | -                              | $7.2 \pm 0.1$ ( $\sim 21\%$ )  | $7.1 \pm 0.1$ ( $\sim 21\%$ )  |
|             | $10^{-7}$ | $11.3 \pm 0.1$ | -                              | $9.0 \pm 0.0$ ( $\sim 20\%$ )  | $9.0 \pm 0.0$ ( $\sim 20\%$ )  |
|             | $10^{-8}$ | $13.7 \pm 0.1$ | -                              | $10.9 \pm 0.0$ ( $\sim 20\%$ ) | $10.8 \pm 0.1$ ( $\sim 21\%$ ) |
| 2-Propanol* | $10^{-6}$ | $9.0 \pm 0.0$  | -                              | $7.1 \pm 0.1$ ( $\sim 21\%$ )  | $7.0 \pm 0.0$ ( $\sim 22\%$ )  |
|             | $10^{-7}$ | $11.3 \pm 0.1$ | -                              | $9.1 \pm 0.1$ ( $\sim 20\%$ )  | $9.0 \pm 0.1$ ( $\sim 20\%$ )  |
|             | $10^{-8}$ | $13.7 \pm 0.1$ | -                              | $11.0 \pm 0.0$ ( $\sim 19\%$ ) | $10.9 \pm 0.0$ ( $\sim 20\%$ ) |
| 2-Hexanol*  | $10^{-6}$ | $9.0 \pm 0.0$  | -                              | $7.0 \pm 0.1$ ( $\sim 23\%$ )  | $7.0 \pm 0.1$ ( $\sim 22\%$ )  |
|             | $10^{-7}$ | $11.0 \pm 0.0$ | -                              | $8.6 \pm 0.1$ ( $\sim 22\%$ )  | $8.6 \pm 0.1$ ( $\sim 22\%$ )  |
|             | $10^{-8}$ | $13.0 \pm 0.0$ | -                              | $10.5 \pm 0.1$ ( $\sim 19\%$ ) | $10.5 \pm 0.1$ ( $\sim 19\%$ ) |
| 1-Heptanol* | $10^{-6}$ | $9.0 \pm 0.0$  | -                              | $6.6 \pm 0.1$ ( $\sim 27\%$ )  | $6.6 \pm 0.1$ ( $\sim 27\%$ )  |
|             | $10^{-7}$ | $10.9 \pm 0.1$ | -                              | $8.3 \pm 0.1$ ( $\sim 24\%$ )  | $8.2 \pm 0.1$ ( $\sim 24\%$ )  |
|             | $10^{-8}$ | $13.0 \pm 0.0$ | -                              | $10.2 \pm 0.1$ ( $\sim 21\%$ ) | $10.3 \pm 0.1$ ( $\sim 21\%$ ) |

| Molecule    | Tol.      | Default guess  | Specific Model                 | Unified Alcohols Model         |
|-------------|-----------|----------------|--------------------------------|--------------------------------|
| 1-Propanol  | $10^{-6}$ | $9.0 \pm 0.0$  | $6.0 \pm 0.1$ ( $\sim 33\%$ )  | $6.4 \pm 0.1$ ( $\sim 29\%$ )  |
|             | $10^{-7}$ | $11.0 \pm 0.1$ | $8.0 \pm 0.0$ ( $\sim 27\%$ )  | $8.1 \pm 0.1$ ( $\sim 27\%$ )  |
|             | $10^{-8}$ | $13.2 \pm 0.1$ | $9.8 \pm 0.1$ ( $\sim 25\%$ )  | $10.0 \pm 0.1$ ( $\sim 24\%$ ) |
| 1-Butanol   | $10^{-6}$ | $9.0 \pm 0.0$  | $6.4 \pm 0.1$ ( $\sim 29\%$ )  | $6.4 \pm 0.1$ ( $\sim 29\%$ )  |
|             | $10^{-7}$ | $11.0 \pm 0.0$ | $8.1 \pm 0.1$ ( $\sim 27\%$ )  | $8.1 \pm 0.1$ ( $\sim 26\%$ )  |
|             | $10^{-8}$ | $13.2 \pm 0.1$ | $10.1 \pm 0.1$ ( $\sim 24\%$ ) | $10.2 \pm 0.1$ ( $\sim 23\%$ ) |
| 2-Butanol   | $10^{-6}$ | $9.0 \pm 0.0$  | $7.2 \pm 0.1$ ( $\sim 20\%$ )  | $6.9 \pm 0.1$ ( $\sim 24\%$ )  |
|             | $10^{-7}$ | $11.1 \pm 0.1$ | $9.0 \pm 0.1$ ( $\sim 19\%$ )  | $8.4 \pm 0.1$ ( $\sim 24\%$ )  |
|             | $10^{-8}$ | $13.2 \pm 0.1$ | $10.9 \pm 0.1$ ( $\sim 18\%$ ) | $10.5 \pm 0.1$ ( $\sim 21\%$ ) |
| 1-Hexanol   | $10^{-6}$ | $9.0 \pm 0.0$  | $6.4 \pm 0.1$ ( $\sim 29\%$ )  | $6.2 \pm 0.1$ ( $\sim 31\%$ )  |
|             | $10^{-7}$ | $10.9 \pm 0.1$ | $8.2 \pm 0.1$ ( $\sim 24\%$ )  | $8.1 \pm 0.1$ ( $\sim 26\%$ )  |
|             | $10^{-8}$ | $13.0 \pm 0.0$ | $10.3 \pm 0.1$ ( $\sim 21\%$ ) | $10.1 \pm 0.1$ ( $\sim 22\%$ ) |
| Ethanol*    | $10^{-6}$ | $9.1 \pm 0.0$  | -                              | $7.0 \pm 0.0$ ( $\sim 23\%$ )  |
|             | $10^{-7}$ | $11.3 \pm 0.1$ | -                              | $8.4 \pm 0.1$ ( $\sim 26\%$ )  |
|             | $10^{-8}$ | $13.7 \pm 0.1$ | -                              | $10.4 \pm 0.1$ ( $\sim 24\%$ ) |
| 2-Propanol* | $10^{-6}$ | $9.0 \pm 0.0$  | -                              | $7.0 \pm 0.0$ ( $\sim 22\%$ )  |
|             | $10^{-7}$ | $11.3 \pm 0.1$ | -                              | $8.4 \pm 0.1$ ( $\sim 25\%$ )  |
|             | $10^{-8}$ | $13.7 \pm 0.1$ | -                              | $10.5 \pm 0.1$ ( $\sim 23\%$ ) |
| 2-Hexanol*  | $10^{-6}$ | $9.0 \pm 0.0$  | -                              | $6.7 \pm 0.1$ ( $\sim 26\%$ )  |
|             | $10^{-7}$ | $11.0 \pm 0.0$ | -                              | $8.4 \pm 0.1$ ( $\sim 24\%$ )  |
|             | $10^{-8}$ | $13.0 \pm 0.0$ | -                              | $10.5 \pm 0.1$ ( $\sim 20\%$ ) |
| 1-Heptanol* | $10^{-6}$ | $9.0 \pm 0.0$  | -                              | $6.4 \pm 0.1$ ( $\sim 29\%$ )  |
|             | $10^{-7}$ | $10.9 \pm 0.1$ | -                              | $8.1 \pm 0.1$ ( $\sim 26\%$ )  |
|             | $10^{-8}$ | $13.0 \pm 0.0$ | -                              | $10.2 \pm 0.1$ ( $\sim 22\%$ ) |

Table S5: Average of the number of iterations obtained using the predicted density matrix as guess for the calculation on the same geometry. The results refer to the (3,8)-models trained targeting the density matrix. The first column specifies the molecule, the second column indicates the convergence tolerance for the SCF procedure, the third column reports the average of the number of iterations obtained using the default guess available in the Gaussian program and in the last two columns we report the average number of iterations obtained with our predicted density matrix as guess, using the specific models and the unified model trained on alcohols, respectively. The values reported in parentheses indicate the percentage of reduction with respect to the iterations required by the default guess to converge. The test molecules with a superscript \* are not included in the training process at all.

## 2 Additional plots

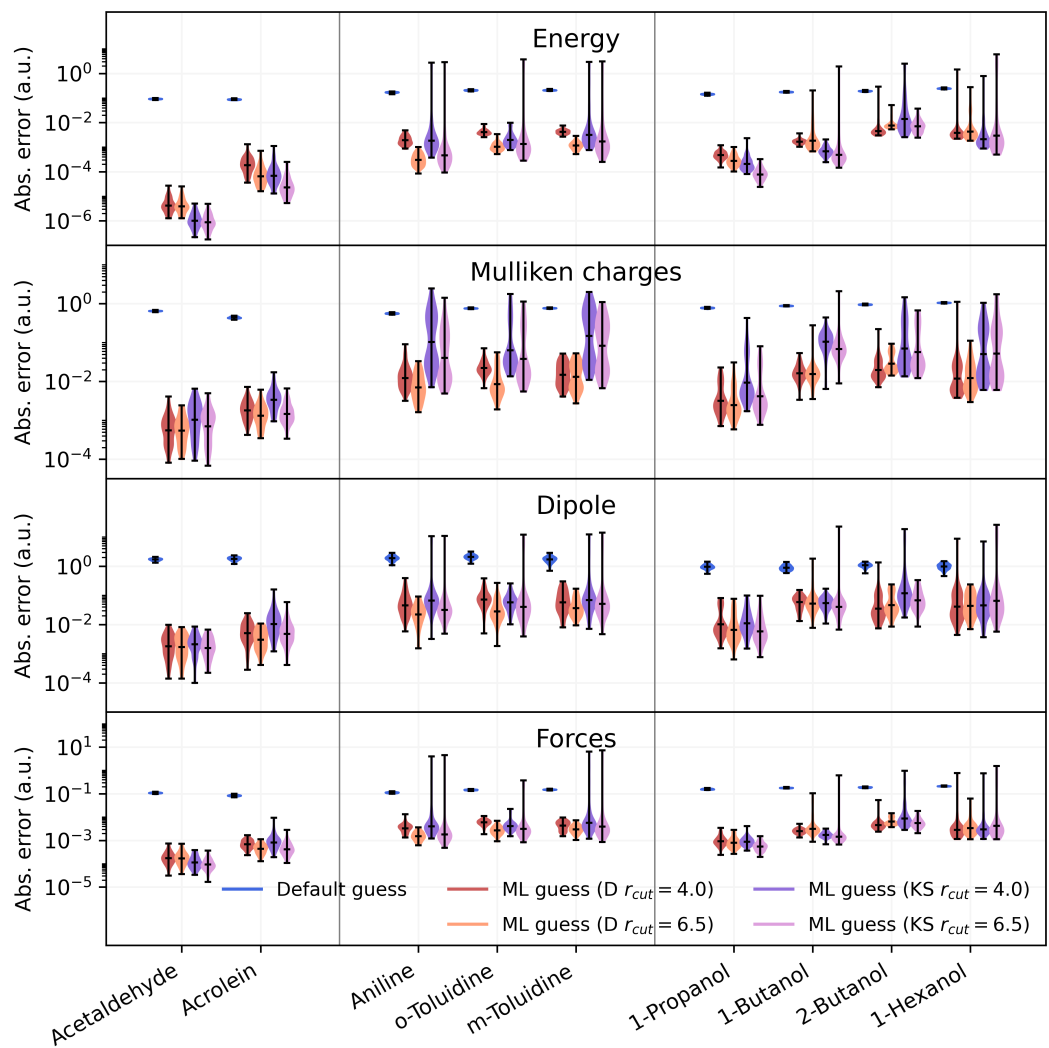

Figure S1: Plot of the error (in logarithmic scale) for energy, Mulliken charges, dipole moment and forces after a single SCF cycle. The blue line represents the default guess provided by Gaussian, red and orange lines refer to models trained on density matrices with cutoff of 4.0 and 6.5 Å, respectively, and violet and pink lines refer to models trained on Kohn-Sham matrices with cutoff of 4.0 and 6.5 Å, respectively.

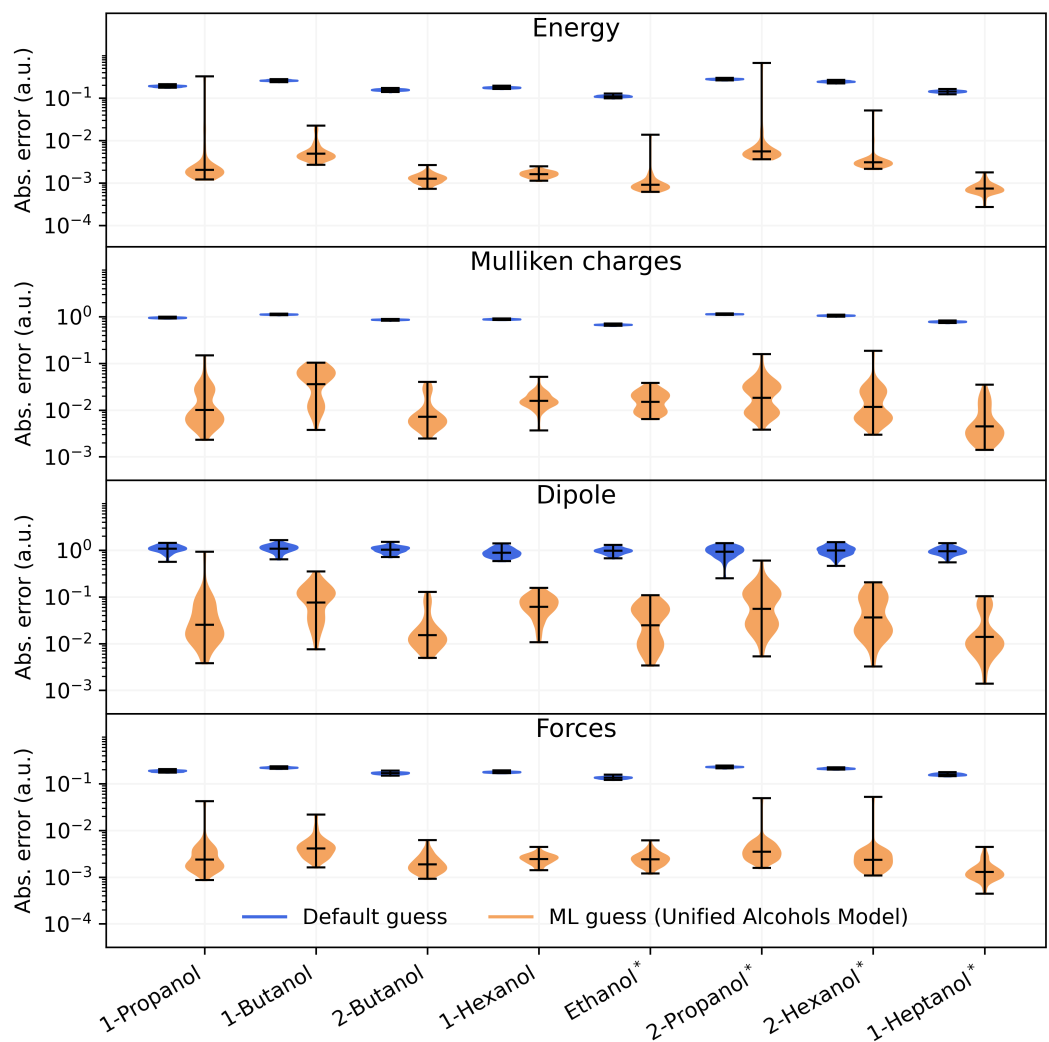

Figure S2: Plot of the error (in logarithmic scale) for energy, Mulliken charges, dipole moment and forces after a single SCF cycle. The blue line represents the default guess provided by Gaussian, while the orange line corresponds to the density matrix predicted using the unified alcohols model. The test molecules with a superscript \* are not included in the training process at all.

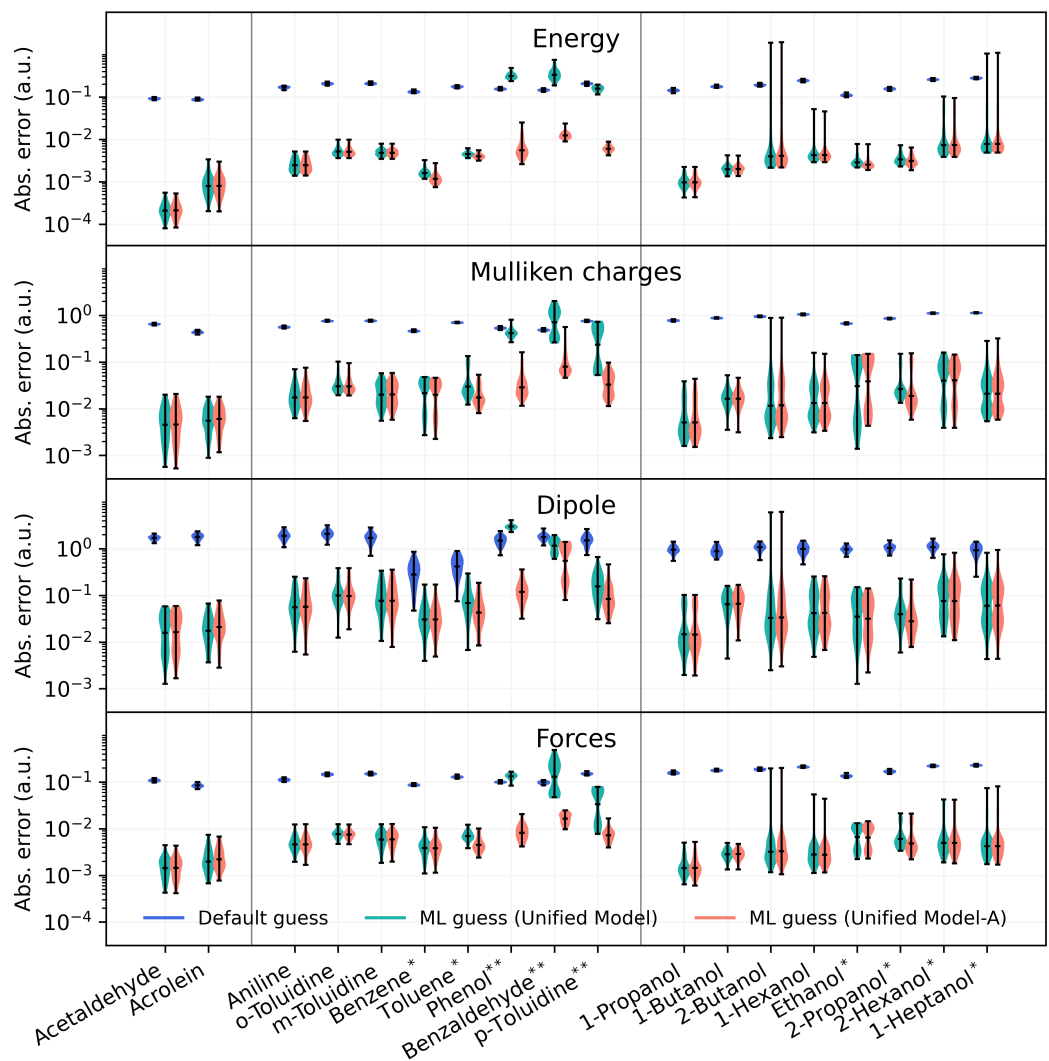

Figure S3: Plot of the error (in logarithmic scale) for energy, Mulliken charges, dipole moment and forces after a single SCF cycle. The blue line represents the default guess provided by Gaussian, while the sea-green and pink lines correspond to the density matrix predicted using the unified model and Unified Model-A, respectively. The test molecules with a superscript \* are not included in the training process at all, and those with \*\* are involved in the training of Unified Model-A, with only 10 frames each included.

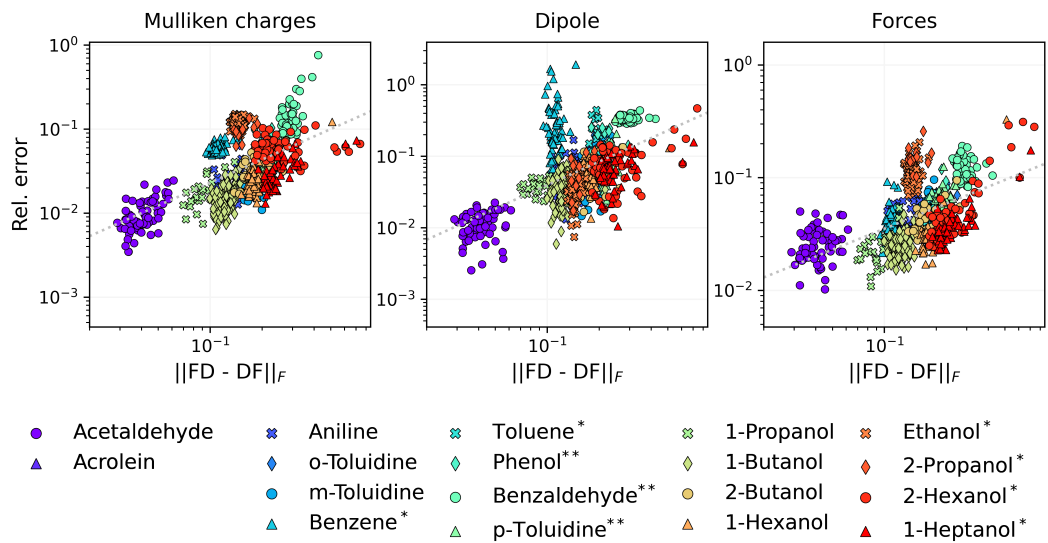

Figure S4: Plot of the Frobenius norm of the commutator between  $F$  and  $D$  versus the relative error in Mulliken charges, dipole moment and atomic forces, obtained after a single SCF cycle, using the density matrix predicted by Unified Model-A as a guess. The test molecules with a superscript  $*$  are not included in the training process at all, and those with  $**$  are involved in the training of Unified Model-A, with only 10 frames each included. As expected, for the dipole moment of benzene, which is close to zero, a clear correlation is not observed.

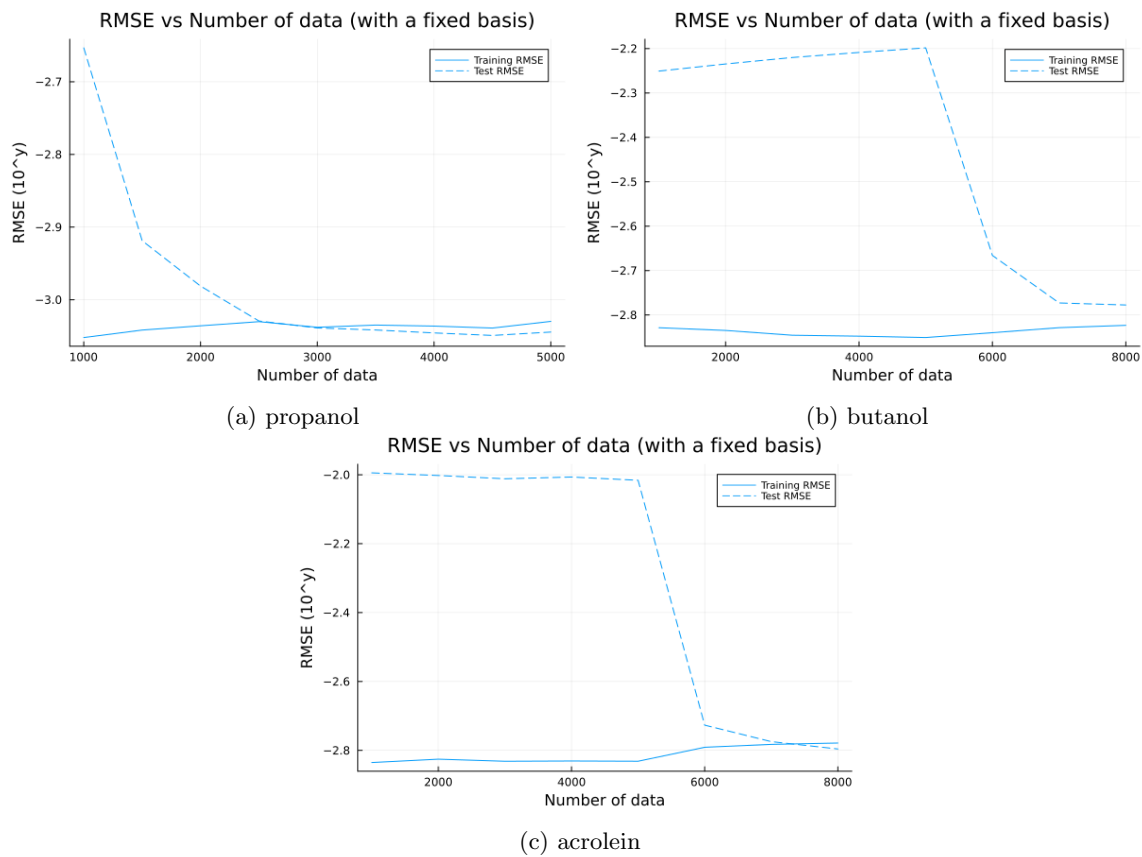

Figure S5: Plot of the relationship between the RMSEs and the number of training configurations for different molecules obtained with a model of moderate size. We pick the amount of training data points for the specific models for each molecule by finding a balance between the training and test set errors.
